# Supplementary material for: Integrative Wrapping System for a Dual-Arm Humanoid Robot
Source: arXiv:2411.08389 source file (2024-11-13)
Supplement: Supplementary file 1 [file appendix.tex]

\section*{APPENDIX}

Appendixes should appear before the acknowledgment.
